# Supplementary material for: Whitepaper on Reusable Hybrid and Multi-Cloud Analytics Service Framework
Source: arXiv:2310.17013 source file (2023-10-25)
Supplement: Supplementary file 1 [file appendix.tex]

\FILE{section-appendix.tex}

\section{Implementation Examples}

This section contains a number of implementation examples that follow the document specifications.

\subsection{Analytics Catalog}
\addcontentsline{toc}{subsection}{Appendix B.1: Anlaytics Catalog}

TBD

\subsection{Analytics Registry}

TBD

\section{Change Log}
\addcontentsline{toc}{section}{Appendix B: Change Log}

If updating document with errata, detail changes made to document.
The updates are recorded in reverse chronological order with the most recent change first.\\

\begin{tabular}{ p{3cm}p{1cm}p{9cm}}
Date            & Initials & Comment \\
\hline
Januarry 2022   & Gregor & merging dictionary terms into the list of terms. \\
December 2021   & RcR 	& \TODO{russel}{Gregor: On the organization of the outline sections and sub sections: 7.2 In my domain, the concept behind the term 'Landscape' would not be related to Specification. I am interested to work on this sub section so I amm looking forward to some clarification on how you see Landscape as a sub of Specification. Depending on the 'vision' of the topics / content for 7.2 and Appendix B, (which I am also interested to work on) they may have some overlap.} \\
September 2021  & GvL & Spelling corrections \\
August 2021     & Gvl & 	Add dictionary \\
                & GvL & Add executive summary \\
                & GvL & Fix introduction \\
                & GvL & Add catalogue \\
                & GvL & Add registry \\
July 2021       & GvL & Integrated notes on Metadata by Russell \\
March 20, 2021  & GvL & First Draft \\
\hline
\end{tabular}
